# Supplementary material for: Observation of collider muon neutrinos with the SND@LHC experiment
Source: arXiv:2305.09383 source file (2023-05-16)
Supplement: Supplementary file 1 [file Appendix.tex]

\clearpage

\appendix*
\section{Background from neutral particles}

Given the low number of simulated neutron and K$^0_L$ events passing all event selection cuts, there is a non negligible statistical uncertainty on the expected background rates. 

Since each energy bin in Tables~\ref{tab:rates} and~\ref{tab:bkg_K0L} has a different scale factor, given by the ratio of the generated events to the predicted interaction rates, a procedure is necessary to combine the statistical uncertainty from the different energy bins taking into account the scale factors.

Distributions of Poisson means, $\lambda$, for a given number of observed events, $k = 0, 1, 2, ...$, are obtained by generating uniformly distributed random $\lambda$ between 0 and 30 (flat prior). From each of these $\lambda$, a random Poisson integer is generated. The posterior distributions of $\lambda$ for each $k$ are obtained by collecting all the $\lambda$ from which an integer equal to $k$ was generated.

To obtain the distribution of the mean number of background events, the distribution of $\lambda$ for each bin is multiplied by the corresponding scale factor and summed. The average number of expected background events, as well as the median and other quantiles are given in Table~\ref{tab:neutral_MC_stats}.
